# Supplementary material for: A Practical Algorithm for Distributed Clustering and Outlier Detection
Source: arXiv:1805.09495 source file (2018-10-11)
Supplement: Supplementary file 1 [file appendix.tex]

\section{Appendix}
\label{sec:appendix}

\subsection{Proof for Corollary~\ref{cor:coreset-quality}}
\label{proof:cor:coreset-quality}

\begin{proof}
  Let $\pi : Q \rightarrow Q$ be the mapping returned by the $\gamma$-approximation algorithm for $(k, t)$-median on $Q$; we thus have $\pi(q)=q$ for all $q \in O$ and $\pi(X\backslash O) = C$. Let $\sigma : X \rightarrow X$ be the mapping returned by Algorithm \ref{alg:coreset} (i.e. $\sigma$ fully determines $Q$). We have that
  \begin{align*}
    \phi(X\backslash O, C) 
    &\leq \sum_{x \in X} d(x, \pi(\sigma(x)))\\
                           &\leq \sum_{x \in X} \left( d(x, \sigma(x)) + d(\sigma(x), \pi(\sigma(x))) \right)\\
                           &= \sum_{x\in X} d(x, \sigma(x)) +  \sum_{x\in X} d(\sigma(x), \pi(\sigma(x))) \\
                           &= \loss(Q) +  \sum_{q\in Q}w_q \cdot d(q, \pi(q)) \\
    &= \loss(Q) +  \sol_{k,t}(Q),
  \end{align*}
  where $\sol_{k, t}(Q)=\sum_{q\in Q}w_q \cdot d(q, \pi(q))$ denotes the cost of the $\gamma$-approximation on $Q$. The corollary follows from  Theorem \ref{thm:coreset} and Lemma \ref{lem:two-level} (set $s = 1$).
\end{proof}
